# Supplementary material for: Phase separation in a mixture of proliferating and motile active matter
Source: arXiv:2506.05288 ancillary file (2025-06-10)
Supplement: Supplementary file 1 [file supplement.pdf]

# Phase separation in a mixture of proliferating and motile active matter
## *Supplemental Material*

Lukas Hupe,[1] Joanna M. Materska,[2] David Zwicker,[1] Ramin Golestanian,[1,3,*] Bartlomiej Waclaw,[2,4,†] and Philip Bittihn[1,‡]

[1] *Max Planck Institute for Dynamics and Self-Organization, Göttingen, Germany*
[2] *Dioscuri Centre for Physics and Chemistry of Bacteria, Institute of Physical Chemistry, Polish Academy of Sciences, Warsaw 01-224, Poland*
[3] *Rudolf Peierls Centre for Theoretical Physics, University of Oxford, Oxford OX1 3PU, United Kingdom*
[4] *School of Physics and Astronomy, The University of Edinburgh, Edinburgh EH9 3FD, United Kingdom*

### CONTENTS

I. Methods 1
  A. Numerical models 1
  B. Reference overlaps 2
  C. Simulation setup 2
  D. Clustering 3
  E. Fitting procedure for effective potential 3

References 3

## I. METHODS

### A. Numerical models

The numerical model used for the two-component simulations is based on the spherocylinder model presented in Ref. 1. Briefly, a cell is modeled as a spherocylinder of radius $R = 0.5$ and length $l$, measured to include the caps. Cells have an internal clock $g$ that grows in time with a rate $\gamma$, which for the growing cells is drawn randomly from the interval $[0.75, 1.25]$. The length of the cell is coupled to $g$ so that cells grow from $l = l^{max}/2$ at $g = 0$ to $l = l^{max}$ at $g = 1$, when they divide into two child cells. Cells interact sterically using forces applied at their closest point, which scale with the 3/2th power of the largest overlap distance, analogous to Hertzian interactions between elastic spheres. The strength of steric interactions is set by the Young's modulus of the cells, here set to $Y = 2.25 \cdot 10^3$.

Equations of motion are overdamped, using mobilities that scale with the cell area reminiscent of dry friction, with translational and rotational mobilities given by

$$\mu^{\text{trans}} = \frac{1}{2R\,l\,\eta} \text{ and } \mu^{\text{rot}} = \frac{12\mu^{\text{trans}}}{4R^2 + l^2}, \tag{S1}$$

with a specific friction $\eta$. In this work, we use $\eta = 0.1875$.

For all growing cells in this work, the division length $l^{max}$ is set to 3. For non-growing cells, the growth rate $\gamma$ is set to zero, and the length is fixed to $l = 2.2R = 1.1$, yielding cells that are only slightly anisotropic. This choice keeps the cell shape close enough to circular to simplify the effective interaction analysis, while still coupling cell orientation to bath dynamics.

Here, this base model is modified in two ways: For non-growing cells, we include a simple self-propulsion force $M \cdot \mathbf{e}_i$ parallel to the cell axis. For growing cells, we add a removal mechanism based on axial stress. Compressive forces acting along the cell axis are measured and integrated using a leaky integrator with memory rate $k_{mem}$, here set to 20, to obtain a smoothed axial force

$$\frac{\mathrm{d}}{\mathrm{d}t}\bar{F}^{int} = k_{mem} \cdot (F^{int} - \bar{F}^{int}) \tag{S2}$$

* ramin.golestanian@ds.mpg.de
† bwaclaw@ed.ac.uk
‡ philip.bittihn@ds.mpg.de

with $F^{int}$ defined as in Ref. 1. When this value exceeds a threshold $F_{\max}$, the cell is removed from the simulation.

Dynamics are integrated using a simple forward Euler integrator, with an adaptive time step regulated to limit maximum cell displacement within a single step. The model is implemented using the InPartS.jl software framework.

The single-component model is built reusing the steric interactions and mobilities from the two-component model, without the growth and removal mechanisms. Since the MSD fits yield an effective self-propulsion velocity (not a force), motility is implemented in this model by directly adding the inferred self-propulsion velocity $v_0\mathbf{e}_i$ to the right-hand side of the equations of motion for the center of mass position of each particle $i$. Rotational and positional diffusion are implemented using an Euler-Maruyama scheme, with stochastic forces added to the positional and orientational degree of freedom. Adhesion is implemented using forces based on the center of mass distance as shown in the main text.

### B. Reference overlaps

To illustrate the meaning of $F_{\max}$, we imagine a cell in between two other cells, each of which overlaps with the original cell by a distance $x$ at its cap. For both interactions, this overlap causes an axial interaction force (of opposite sign for the two cells) according to the Hertzian interaction law (Ref. 1, Eq. 26), with a magnitude of

$$F^{ov} = \frac{Y}{2}\sqrt{\frac{R}{2}}x^{3/2}. \tag{S3}$$

To link the overlap distance $x$ to the internal axial compression measured by the cell we use Eq 11 and 15 of Ref. 1, with

$$F^{int} = 2F^{ov} = Y\sqrt{\frac{R}{2}}\,x^{3/2} \tag{S4}$$

$$\Rightarrow \quad x = \left(\frac{2(F^{int})^2}{Y^2 R}\right)^{1/3}. \tag{S5}$$

Thus, one force unit corresponds to a reference overlap $x$ of approximately $9.24 \cdot 10^{-3}$, or about 1.85 % of the cell radius. For the four values of $F_{\max}$ used in the main text, the reference overlaps are as given in Table S1.

| $F_{\max}$ | $x$ | $x/R$ |
|---|---|---|
| 7 | $33.8 \cdot 10^{-3}$ | 6.77 % |
| 10 | $42.9 \cdot 10^{-3}$ | 8.58 % |
| 15 | $56.2 \cdot 10^{-3}$ | 11.2 % |
| 20 | $68.1 \cdot 10^{-3}$ | 13.6 % |

TABLE S1. Reference overlaps for given $F_{\max}$

### C. Simulation setup

Two-component simulations are initialized with cells of random age at an area density of approximately 0.85, with 27.5 % of the cell area taken up by motile cells. Dense initial conditions are created by initializing randomly oriented cells on a grid in a larger domain, then dynamically reducing the domain size to the target size.

Full-system simulations, both with the two- and single-component models, are run in periodic domains of size $80 \times 80$, integrated for $2 \cdot 10^4$ time units (corresponding to approximately the same number of generations in the growing phase). System snapshots are saved for analysis every 6.25 time units. For the tracer simulations used to infer the effective model parameters, simulations are run on smaller domains of size $40 \times 40$ for $10^5$ time units, with tracer positions saved every snapshots.

Full system simulations of both the single-component and two-component model were repeated for four different initial conditions and random number seeds. For single tracer simulations we used two different realisations, two-tracer realisations were repeated 28 times.

### D. Clustering

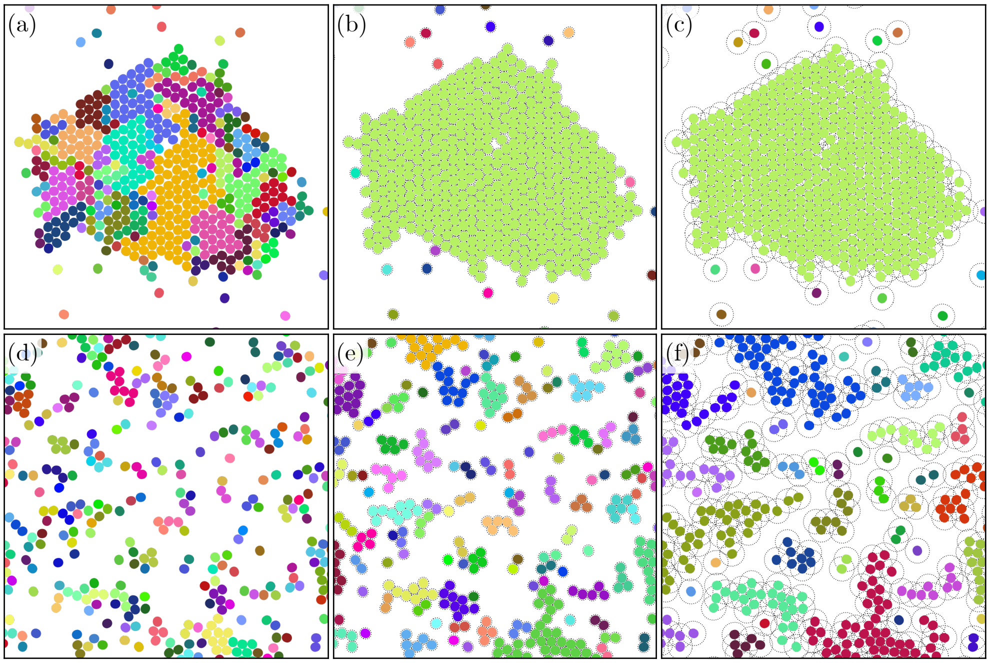


FIG. S1. (a) Snapshot of a single component simulation at parameters equivalent to $F_{\max} = 2$ and $M = 0$ with cells coloured by identified clusters, using cell overlap as the adjacency criterion. (b) Same as panel a, but considering cells within an edge-to-edge distance of 0.1 cell diameters as adjacent. Dotted black lines around cells indicate maximum edge-to-edge distance (c) Same as panel b, but using the range of the adhesion law as maximum edge-to-edge distance. (d–f) Same as panels a to c, but for parameters equivalent to $F_{\max} = 7$ and $M = 1.98$.

Clusters are identified by building a graph of non-growing cells, where every cell is connected to every adjacent cell, and identifying the connected components of the graph. For the two-component model, two cells must have non-zero overlap in order to be directly connected in the graph. In the single component model non-zero cell overlaps are much rarer as the adhesion force only applies to non-overlapping cells. As illustrated in Fig. S1a, this means that using non-zero overlap as the adjacency criterion produces small, fragmented clusters. On the other hand, using a too generous adjacency range, e.g. the entire interaction range including the adhesion law as in Figs. S1c and S1f produces spurious clusters in the dilute regime. We therefore choose to consider cells with an edge-to-edge distance of up to 0.1 cell diameters adjacent, which we find to be a good compromise in both limits (Figs. S1b and S1e).

### E. Fitting procedure for effective potential

The simple linear adhesion force introduced in the main text is parameterized by the potential well depth $V_1$, barrier height $V_2$ and barrier position $r_2$. We fit parabolas to small regions around the two extrema in the numerical effective potentials to obtain estimates for these quantities.

When applying the potential inference method to two single-component cells, we notice that the well produced by the potential inference is slightly shallower than prescribed. This is an effect of the slight anisotropy of the non-motile cells, which causes the steric repulsion and adhesion regimes to overlap in the range from $r = 1.0$ to $1.1$, thus decreasing the depth of the potential well. To correct for this effect, we apply a correction to $V_1$ in order to match the inferred well depths in single- and two-component test simulations.

[1] L. Hupe*, Y. G. Pollack*, J. Isensee, A. Amiri, R. Golestanian, and P. Bittihn, A minimal model of smoothly dividing disk-shaped cells (2024), arXiv:2409.01959 [cond-mat].

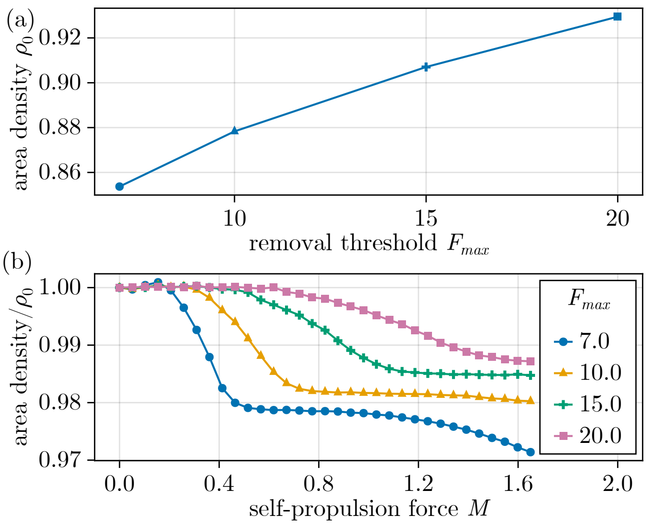


FIG. S2. (a) Area density at zero motility $\rho_0$ as a function of $F_{\max}$ (b) Area density as a function of motility $M$ for different $F_{\max}$, normalized with $\rho_0$

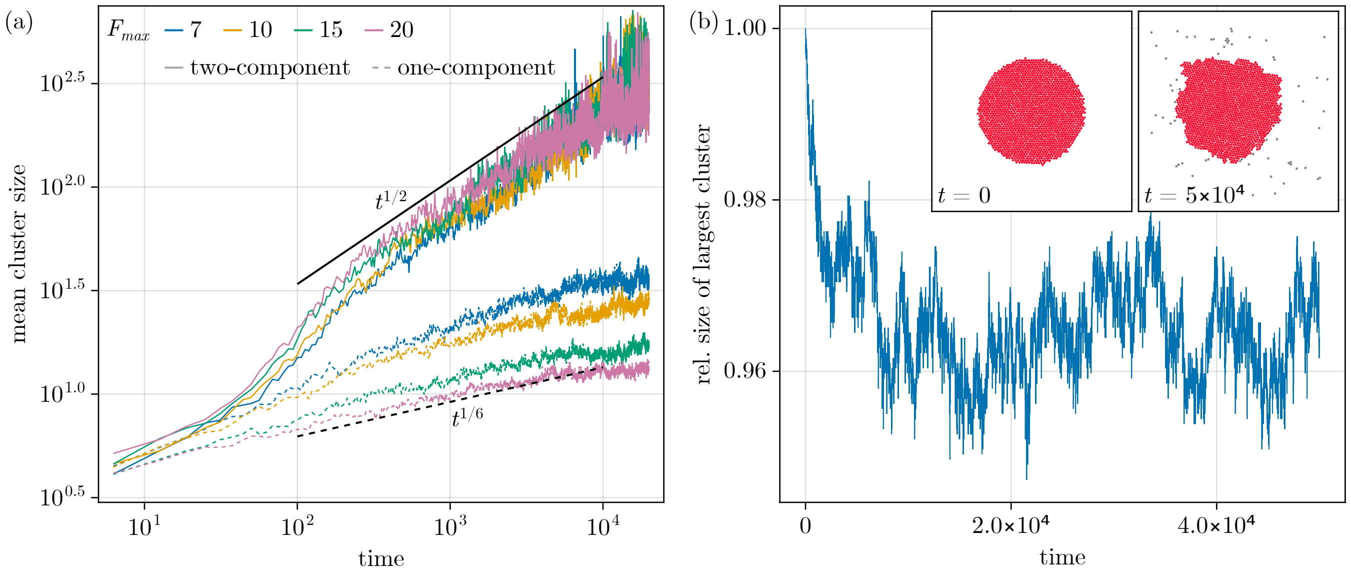


FIG. S3. (a) Mean cluster size time series in two- and one-component simulations for zero motility. The two-component model phase-separates faster. (b) Time series of the relative largest cluster size in a one-component simulation initialized with a single dense cluster of 1690 particles, for parameters corresponding to zero motility and $F_{\max} = 10$. Insets show simulation snapshots at beginning and end of the simulation. The fact that the cluster does not break up might indicate that coarsening in the one-component model might continue to full phase separation as in the two-component model, albeit very slowly.

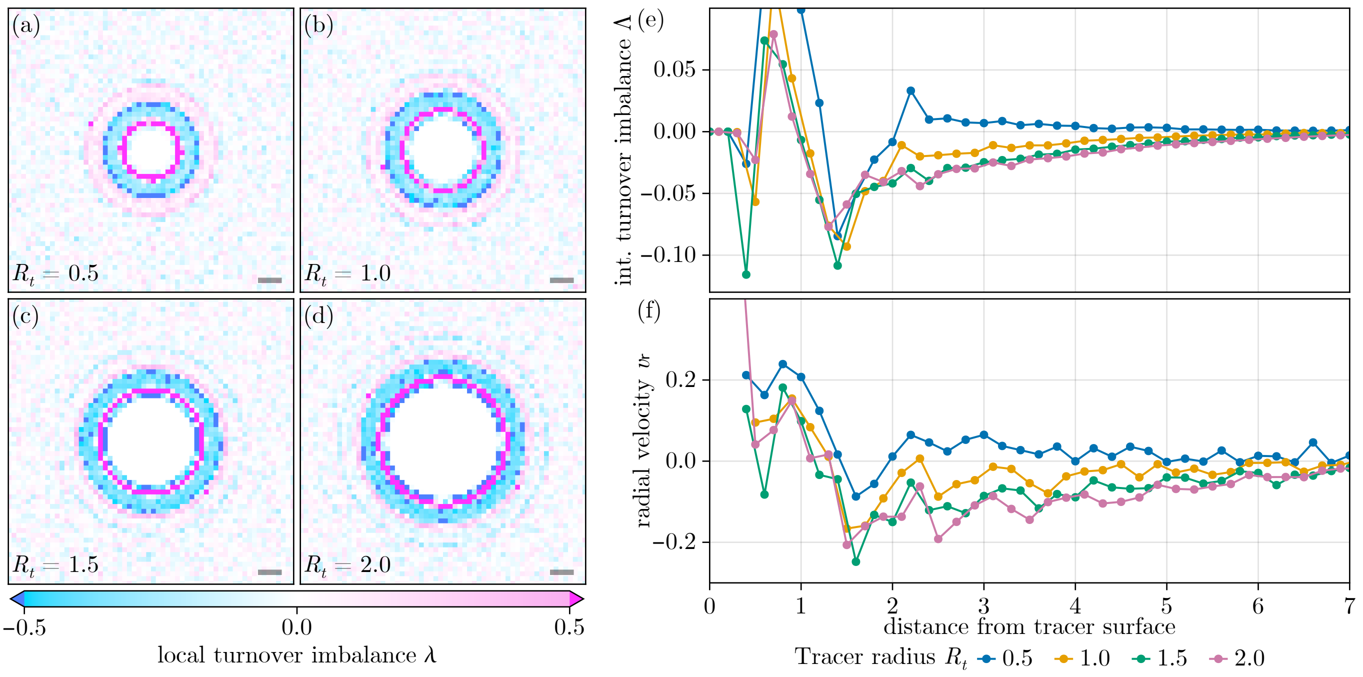


FIG. S4. (a–d) Local turnover imbalance heatmaps for tracers of varying radii, from $r = 0.5$ (top left) to 2.0 bottom right. (e) Integrated turnover imbalance around a tracer of varying radius (see legend) as a function of distance from the tracer surface. (f) Radial velocity of bath particles around a tracer of varying radius as a function of distance from the tracer surface.
